# Supplementary material for: Rectifying the Shortcut Learning of Background for Few-Shot Learning
Source: arXiv:2107.07746 source file (2022-01-05)

Original image

Top-3 crops

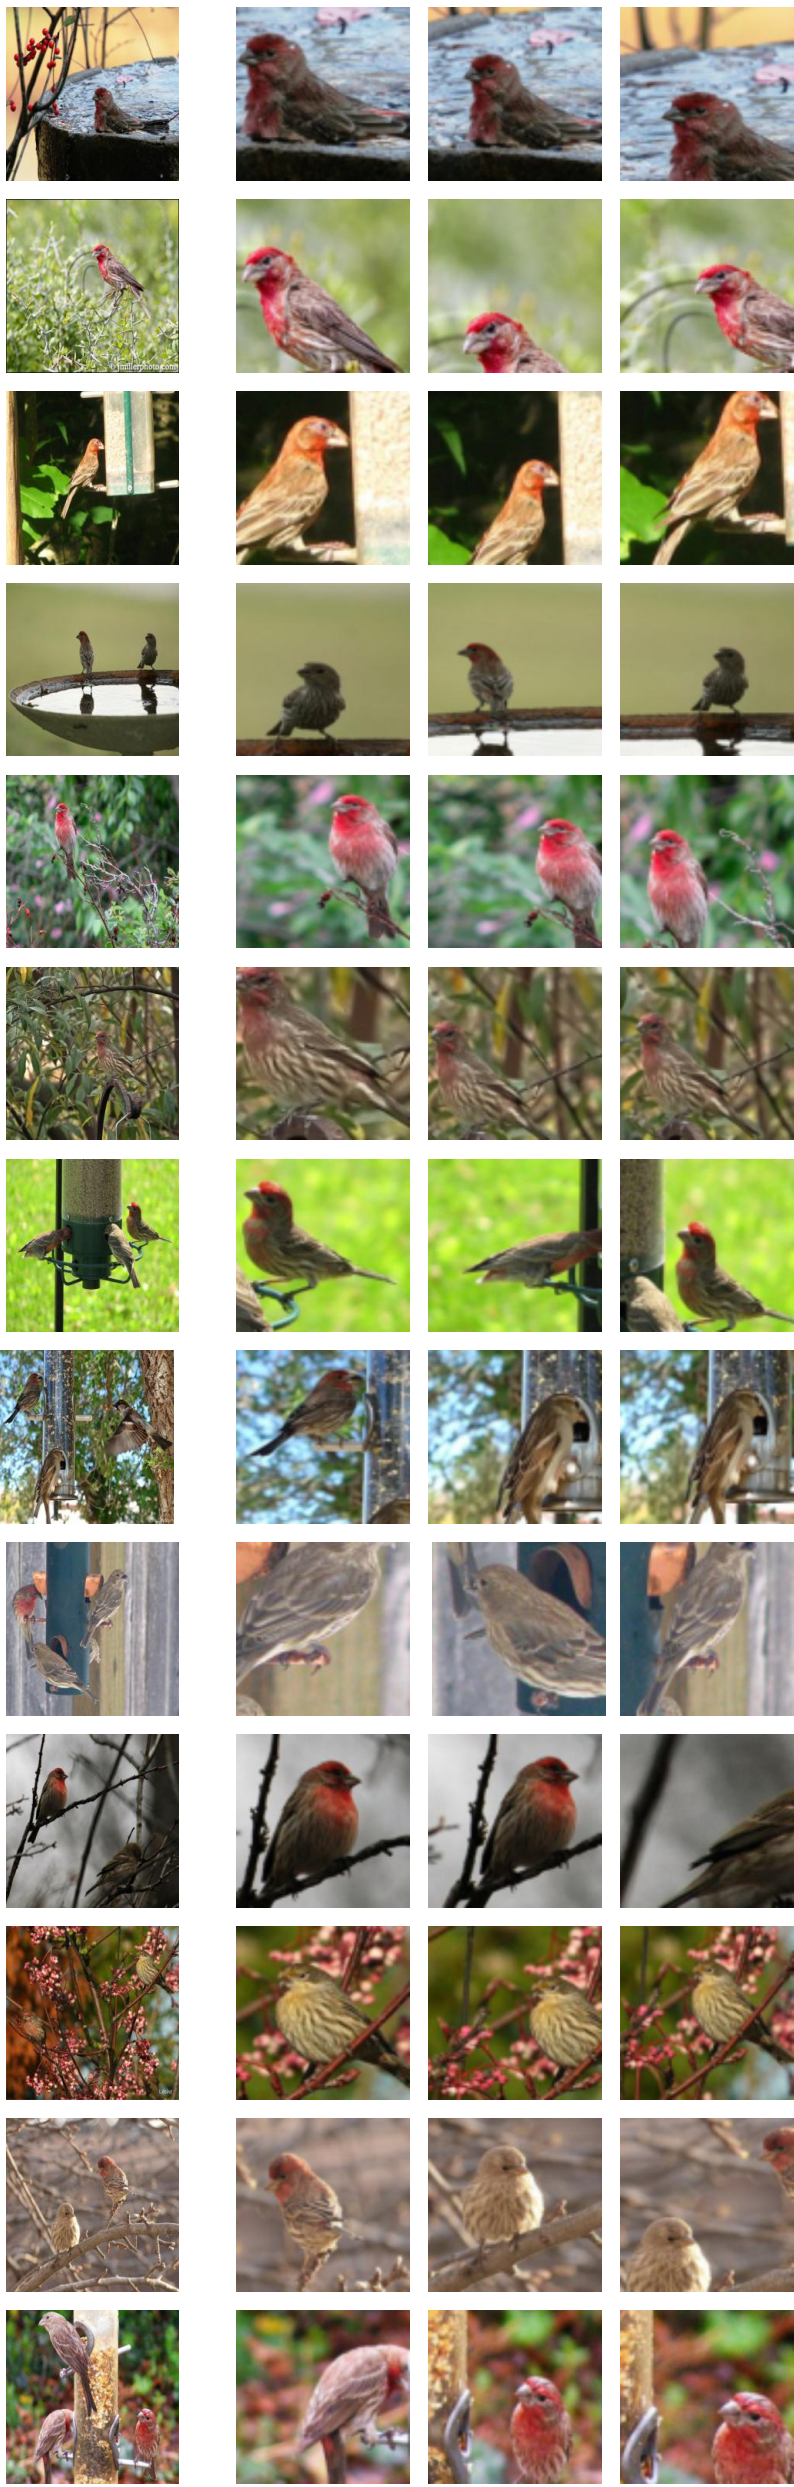

Original image

Top-3 crops

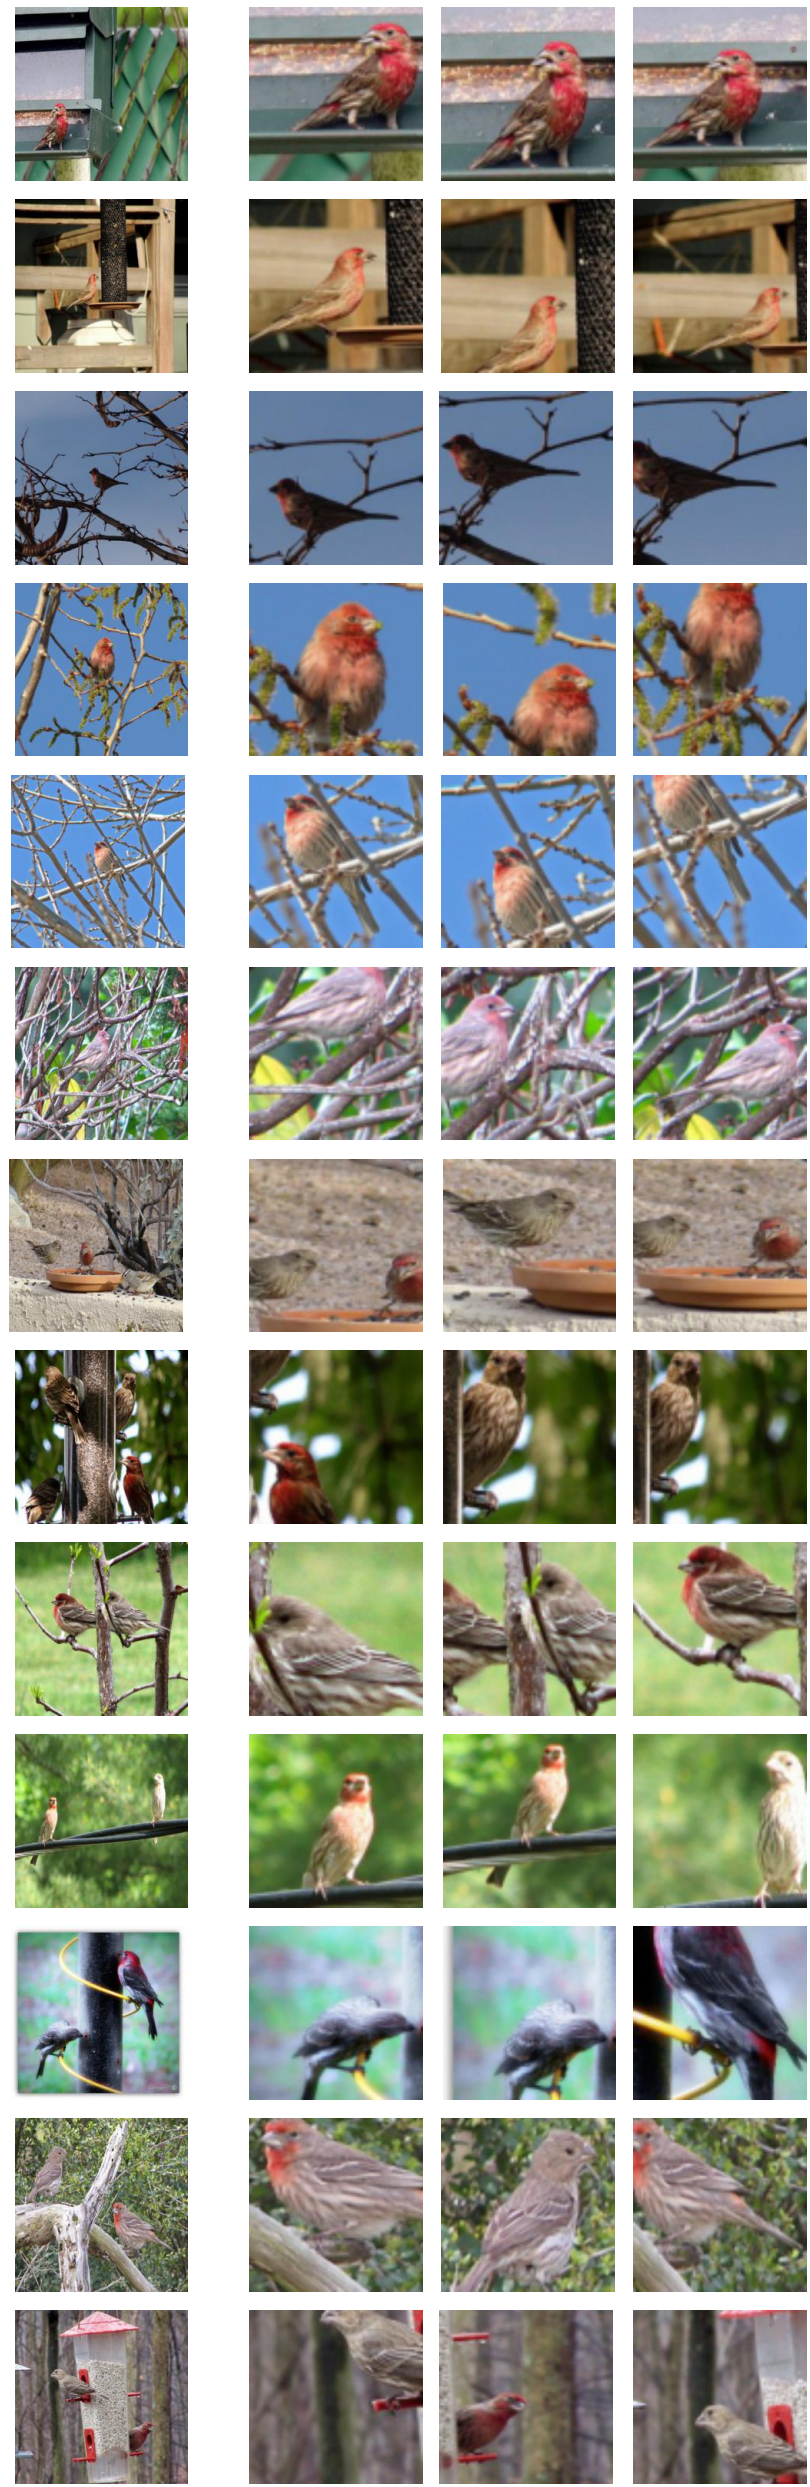

Supplement: Supplementary file 1 [file appendix_pretrain_1.pdf]
